# Supplementary material for: mmFUSION: Multimodal Fusion for 3D Objects Detection
Source: arXiv:2311.04058 source file (2023-11-07)
Supplement: Supplementary file 1 [file X_suppl.tex]

%\clearpage
\setcounter{page}{1}
%\maketitlesupplementary
\section{Additional Details about Experiments}
\textbf{Loss Functions.}
Our total loss is the sum of three losses expressed as:
\begin{equation}
    \mathcal{L} = \mathcal{L}_{cls} + \mathcal{L}_{reg} + \mathcal{L}_{dir}
\end{equation}
where $\mathcal{L}_{cls}$ denotes the focal loss \cite{lin2017focal} for classification, which balances the positive and negative sample with setting $\alpha = 0.25$ and $\gamma = 2.0$.
The $\mathcal{L}_{reg}$ denotes smooth L1 loss \cite{girshick2015fast} for bounding box regression with setting $\beta=1/9$ and loss weight to 2.
Finally, $\mathcal{L}_{dir}$ denotes the cross entropy loss for direction classification with setting loss weight to 0.2.

\textbf{Train Process}
We train our proposed mmFUSION framework in an end-to-end manner following all the settings mentioned in the main paper. We report the top performance in the last 5 epochs for stable comparison. 
%Figure \ref{fig_losses_kitti} and \ref{fig_losses_nuscenes} show plots for all losses during mmFUSION training on the KITTI and NuScenes datasets respectively. 
Figure \ref{Car3dAP40_kitti} shows an evaluation comparison of our method with the baseline at each epoch for 3D detection considering different difficulty levels as defined by KITTI (Car only). In Figure \ref{NDS_mAP_nuscenes} , we show mAP and NDS during the training of mmFUSION on nuscenes data for 31 epochs (all classes).
%Similarly, \ref{NDS_mAP_nuscenes} shows an evaluation comparison of NDS and mAP of our method with a baseline on nuscenes data (all classes)

 %left bottom right top
 %\begin{figure}[ht!]
 %    \centering
 %    \includegraphics[trim=0.5cm 0 0.5cm 0 , width=9cm,height=8.2cm,keepaspectratio]{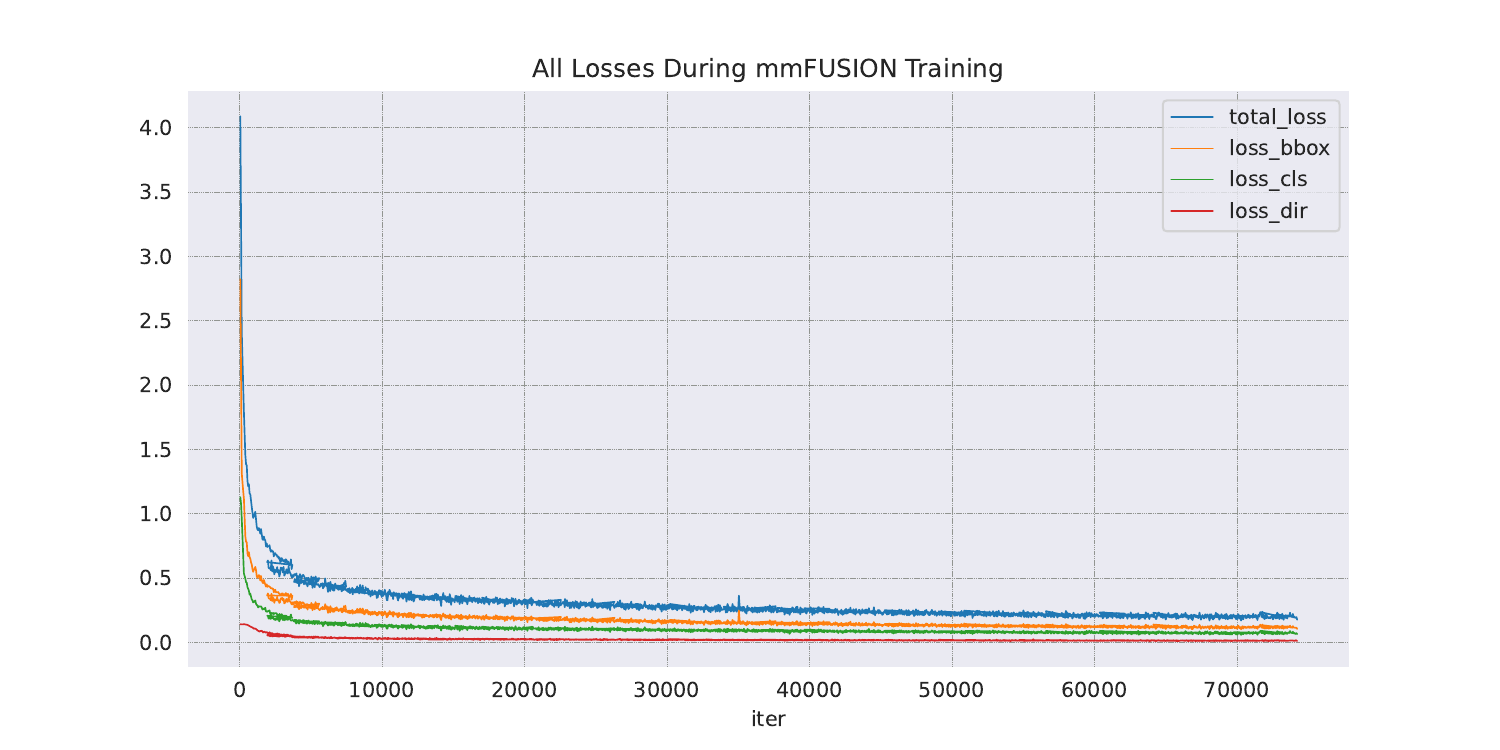}
 %    \caption{Losses curves during mmFUSION training on KITTI}
 %    \label{fig_losses_kitti}
 %\end{figure}

 %left bottom right top
%\begin{figure}[ht!]
%     \centering
%     \includegraphics[trim=0.5cm 0 0.5cm 0 , width=9cm,height=8.2cm,keepaspectratio]{figs/supp_material/mmFUSION_all_loss.pdf}
%     \caption{Losses curves during mmFUSION training on NuScenes}
%     \label{fig_losses_nuscenes}
% \end{figure}

 %left bottom right top
 \begin{figure}[h]
     \centering
     \includegraphics[trim=0.5cm 0 0.5cm 0 , width=9cm,height=8.2cm,keepaspectratio]{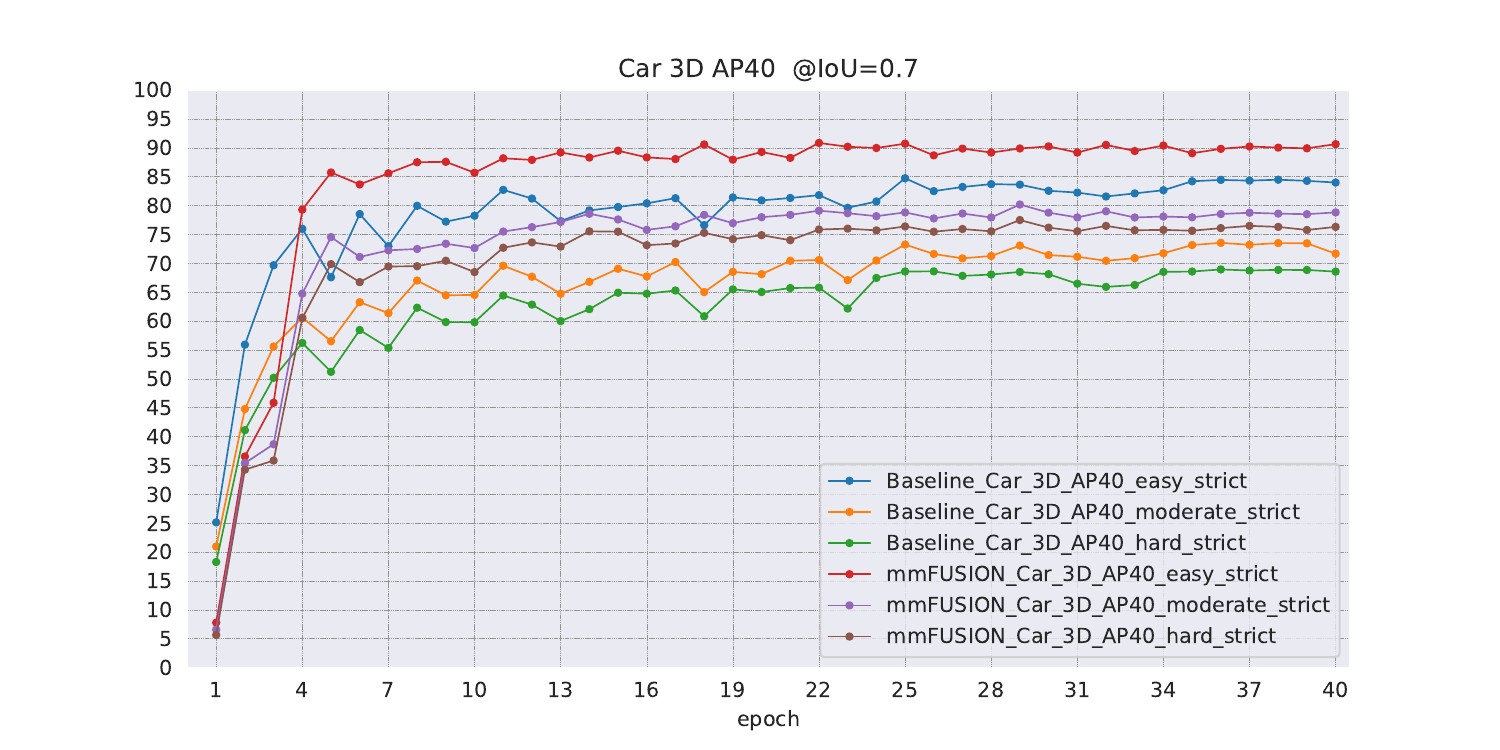}
     \caption{Evaluation comparison of mmFUSION with baseline at each epoch on KITTI.}
     \label{Car3dAP40_kitti}
 \end{figure}

 %left bottom right top
 \begin{figure}[h]
     \centering
     \includegraphics[trim=0.5cm 0 0.5cm 0 , width=9cm,height=8.2cm,keepaspectratio]{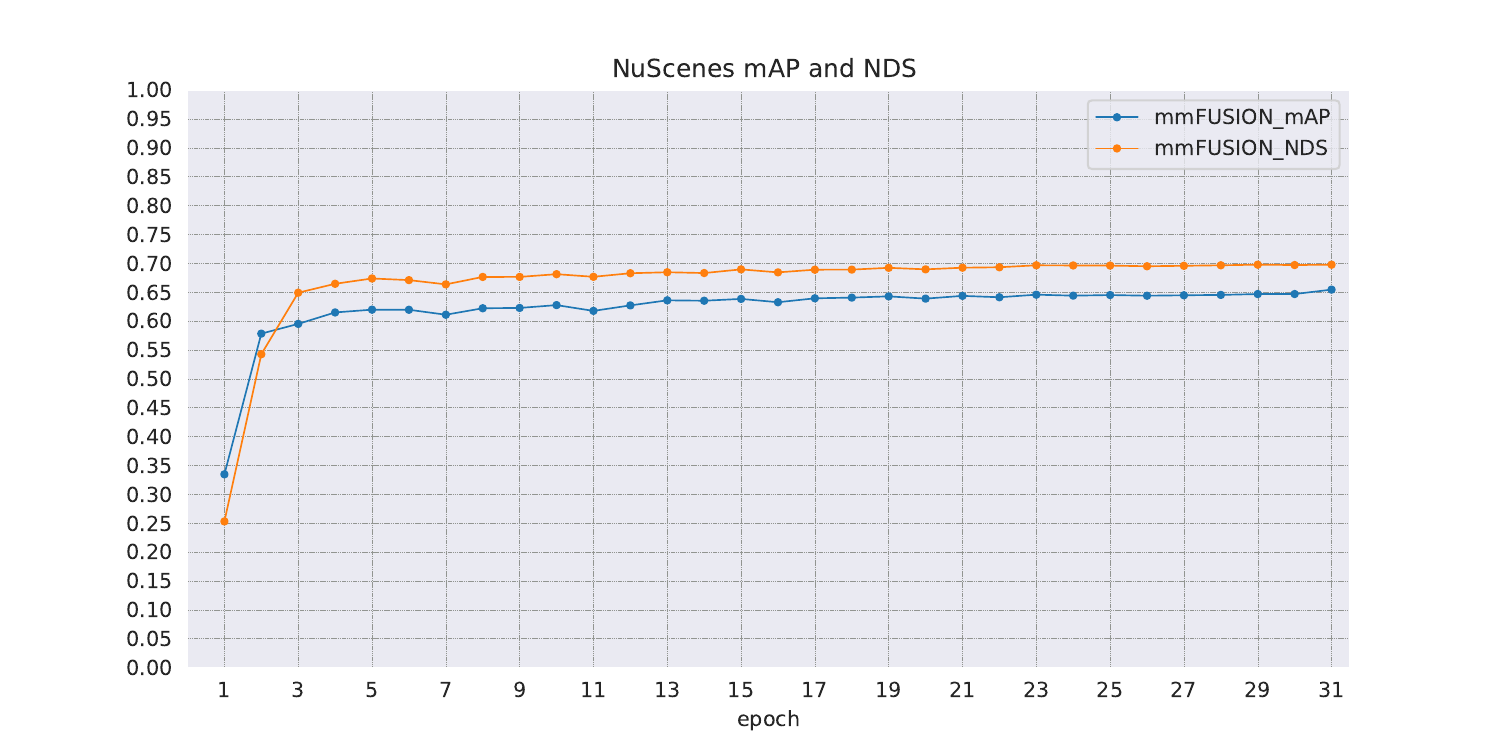}
     \caption{Evaluation of mmFUSION at each epoch on NuScenes.}
     \label{NDS_mAP_nuscenes}
 \end{figure}

\textbf{Test Process}

We report precision-recall (PR) curves in Figure \ref{fig:precision_recall_onkittiTest} on the KITTI test set for the car category. Our mmFUSION results on the test set are better than other fusion schemes as described in the main paper. These test results have been reported after submitting our predictions to the online KITTI leaderboard.

\subsection{Extended Visualization}
We extend our visualization on another KITTI example in Figure \ref{fig:overll_qualitative_example2}, where the order is the same as in its first example. %Next in Figure \ref{fig:overall_qualitative_example_nuscenes1}, we further visualize mmFUSION detection on NuScenes example,  comparing with \cite{} it is interesting to see mmFUSION correctly detects objects on this competitive scene.

\begin{figure*}[h!]
\centering
    \begin{subfigure}[b]{0.25\textwidth}
         \centering
         \includegraphics[trim=1cm 0 0.3cm 1cm,width=\textwidth]{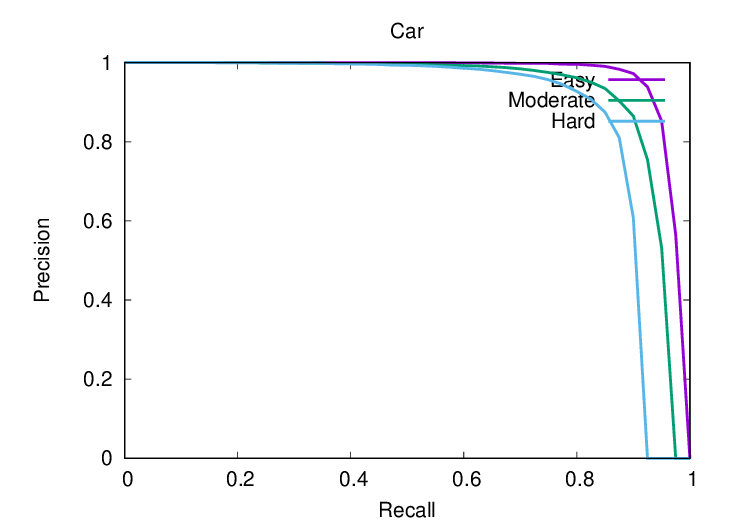}
         \caption{Car: Detection}
         \label{fig:y equals x}
     \end{subfigure}
     %\hspace{0.4cm}
     \hfill
     \begin{subfigure}[b]{0.225\textwidth}
         \centering
         \includegraphics[trim=2cm 0 0.5cm 1cm, width=\textwidth]{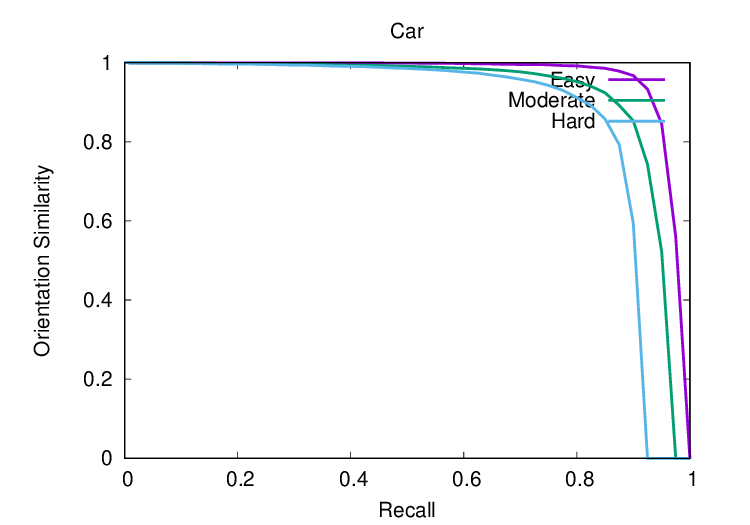}
         \caption{Car: Orientation}
         \label{fig:three sin x}
     \end{subfigure}
     %\hspace{0.4cm}
     \hfill
     \begin{subfigure}[b]{0.23\textwidth}
         \centering
         \includegraphics[trim=1.7cm 0 0.3cm 1cm,width=\textwidth]{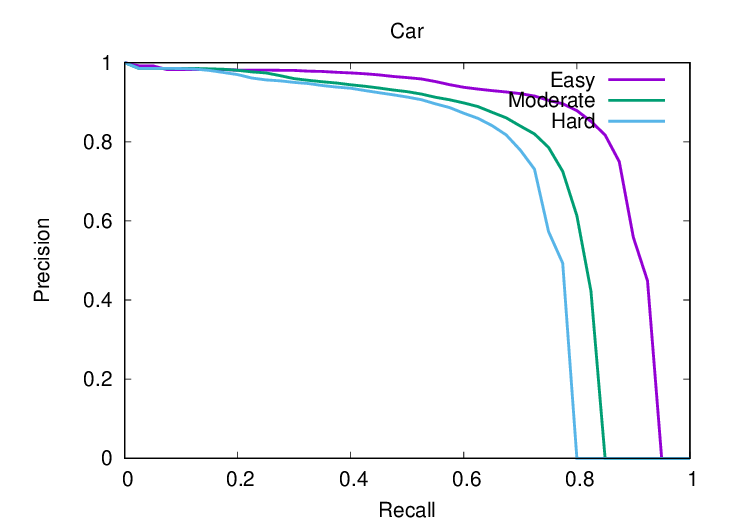}
         \caption{Car: 3D Detection}
         \label{fig:five over x}
     \end{subfigure}
     %\hspace{0.4cm}
     \hfill
     \begin{subfigure}[b]{0.21\textwidth}
         \centering
         \includegraphics[trim=2cm 0 1cm 1cm,width=\textwidth]{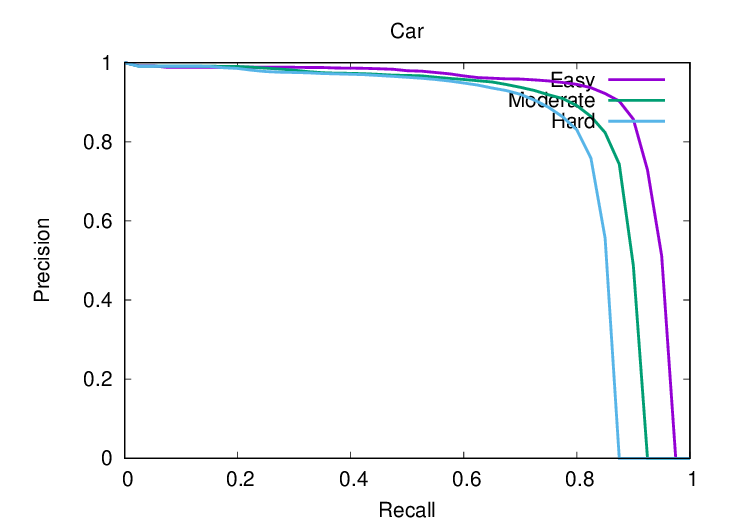}
         \caption{Car: Bird's Eye View}
         \label{fig:five over x}
     \end{subfigure}
    \caption{Precision-Recall curves of mmFUSION on the KITTI \textit{test} set.}
    \label{fig:precision_recall_onkittiTest}
\end{figure*}

\begin{figure*}[h!]
    \centering
    \begin{subfigure}[b]{0.495\textwidth}
            \centering
            % raw image
            \begin{subfigure}[b]{1\textwidth}
                \centering
                \includegraphics[width=\textwidth]{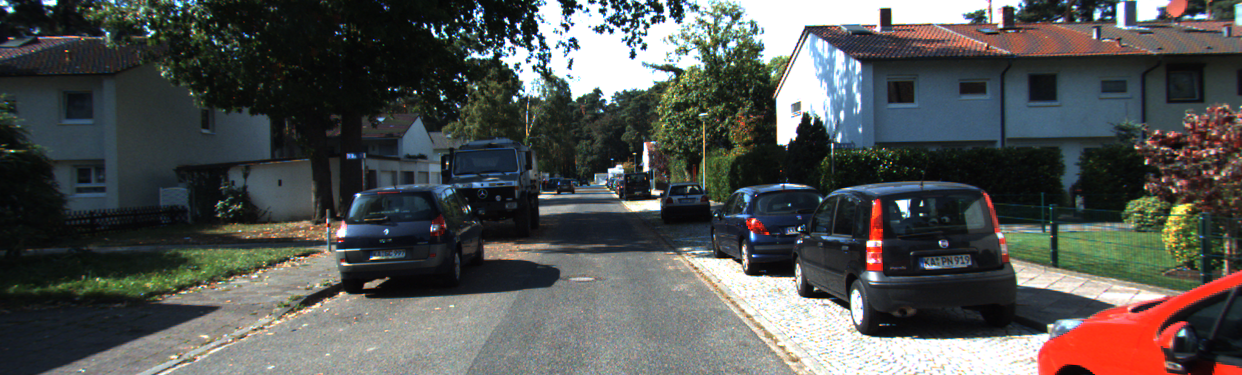}
            \end{subfigure}
            % lidar points
            \begin{subfigure}[b]{1\textwidth}
                \centering
                \includegraphics[width=\textwidth]{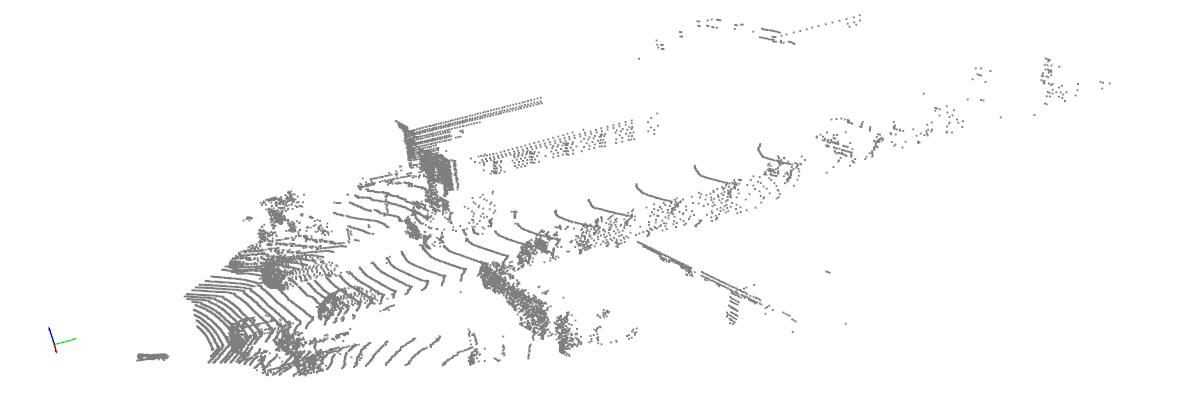}
            \end{subfigure}
            % projected points on image
            \begin{subfigure}[b]{1\textwidth}
                \centering
                \includegraphics[width=\textwidth]{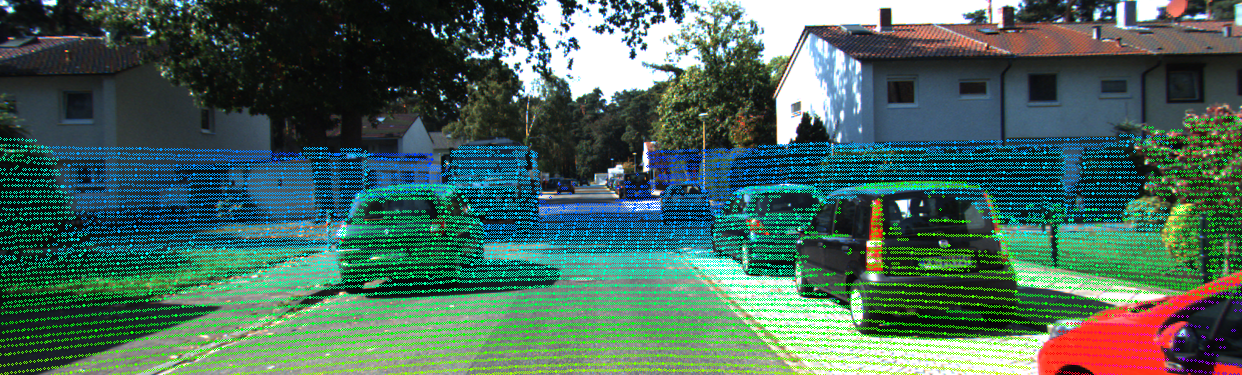}
             %\vspace{0.05cm}
            \end{subfigure}
           
            % projected gt 3D boxes on image
            \begin{subfigure}[b]{1\textwidth}
                \centering
                \includegraphics[width=\textwidth]{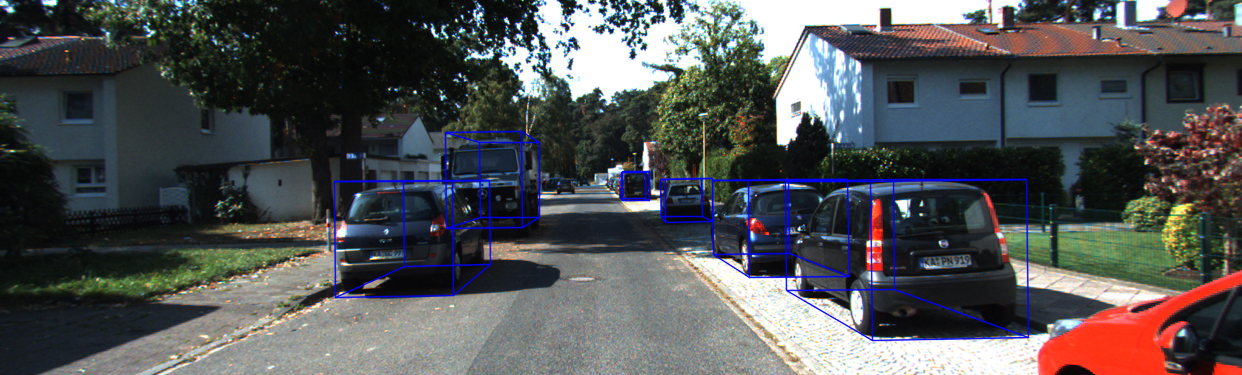}
            \end{subfigure}
            % projected predicted 3D boxes on image
            \begin{subfigure}[b]{1\textwidth}
                \centering
                \includegraphics[width=\textwidth]{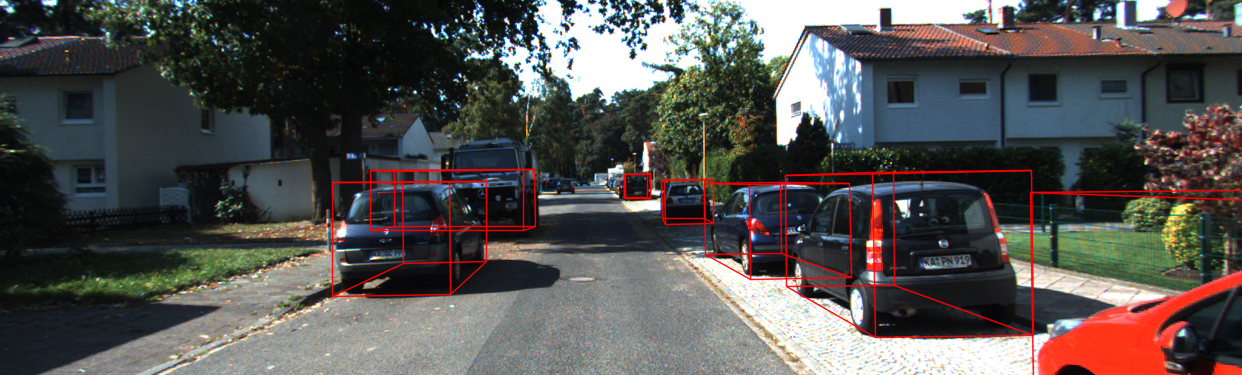}
            \end{subfigure}

    \end{subfigure}
    %\hspace{-0.1cm}
    \begin{subfigure}[b]{0.45\textwidth}
             \centering
            % img low spatial shape
            \begin{subfigure}[b]{0.95\textwidth}
                \centering
                \includegraphics[width=\textwidth]{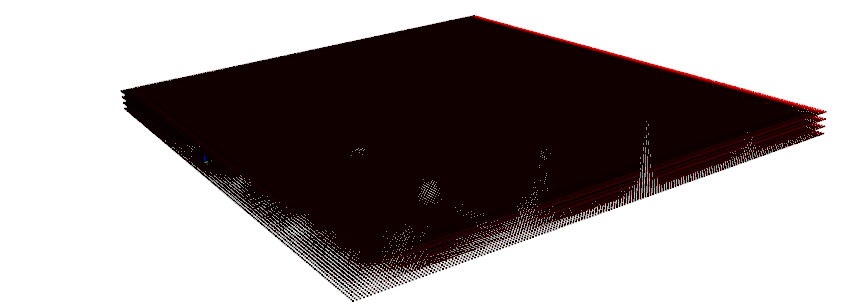}
            \end{subfigure}
            % lidar low spatial shape
            \begin{subfigure}[b]{0.95\textwidth}
                \centering
                \includegraphics[width=\textwidth]{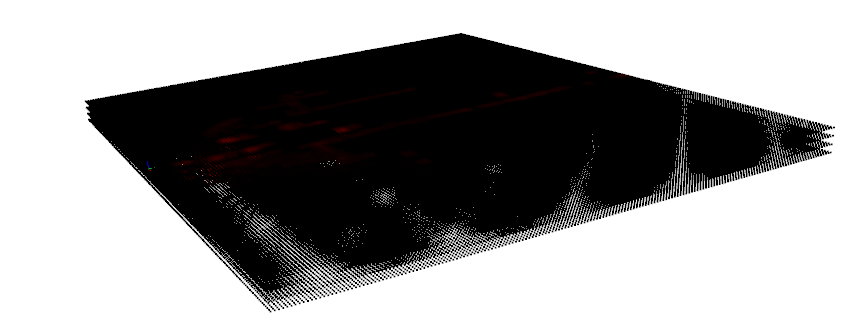}
            \end{subfigure}
            % multimodality low spatial shape
            \begin{subfigure}[b]{1\textwidth}
                \centering
                \includegraphics[width=\textwidth]{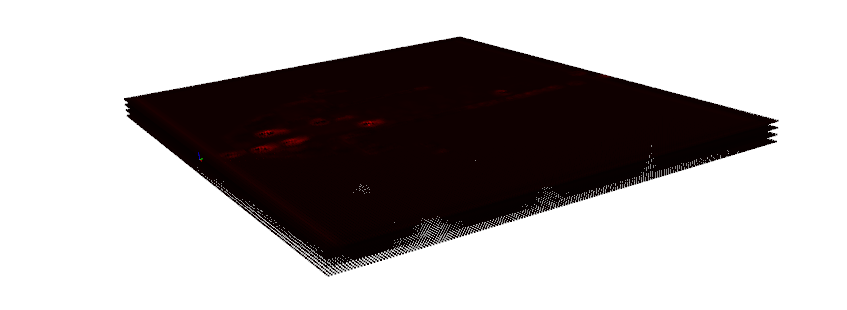}
                %\vspace{0.05cm}
            \end{subfigure}
            % drawn gt boxes on multimodality low spatial shape
            \begin{subfigure}[b]{1\textwidth}
                \centering
                \includegraphics[width=\textwidth]{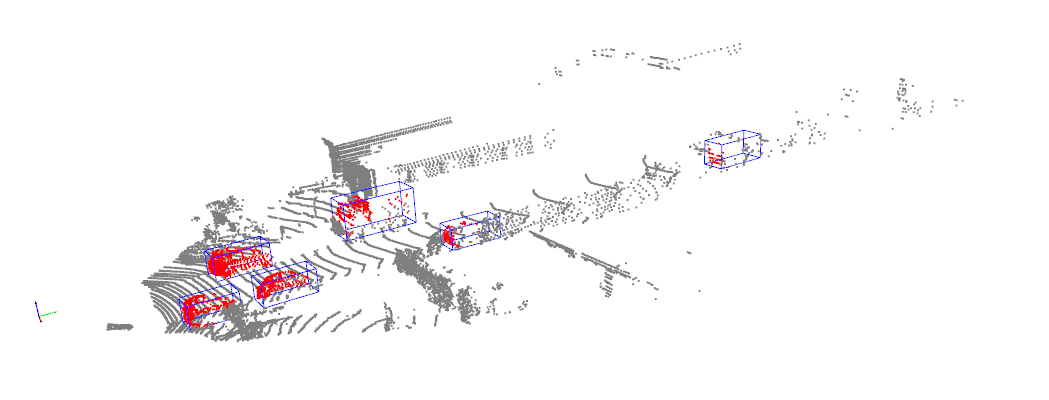}
            \end{subfigure}
            % drawn pred boxes on multimodality low spatial shape
            \begin{subfigure}[b]{1\textwidth}
                \centering
                \includegraphics[width=\textwidth]{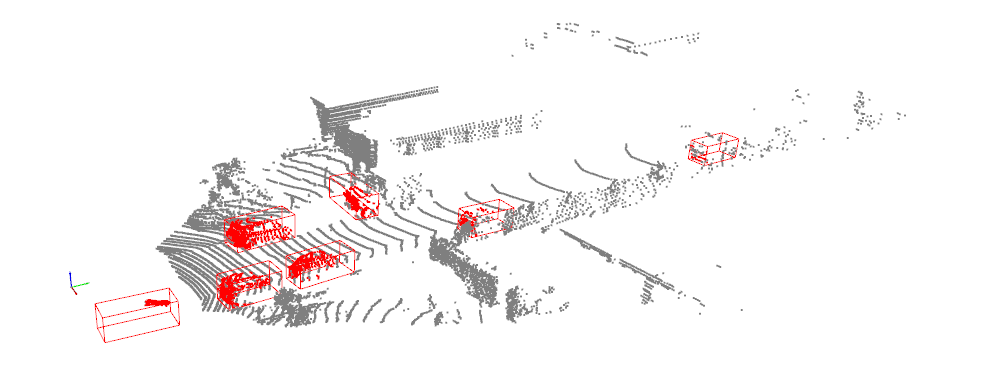}
            \end{subfigure}
            
    \end{subfigure}
    \caption{Extended visualizations with another KITTI example, order is same as the first example in the main paper}
%    \caption{Examples of the proposed low spatial shape on KITTI \textit{val} set. The blue points indicate the projected features in low spatial shape while green points show LiDAR points.}
    \label{fig:overll_qualitative_example2}
\end{figure*}
